# Supplementary material for: The ObjectFolder Benchmark: Multisensory Learning with Neural and Real Objects
Source: arXiv:2306.00956 source file (2023-06-01)
Supplement: Supplementary file 1 [file supplementary_video.tex]

% Details of the Supplementary video
%\subsection{Supplementary Video}\label{sec:supplementary video}

%In the supplementary video, we show 1) motivations of multisensory object modeling and understanding, 2) examples of the multisensory data collected for one object in \namereal, 3) examples of multisensory data collection process for all 100 objects in \namereal, and 4) an overview of the 10 multisensory object-centric learning tasks presented in the \name suite.
